# Supplementary material for: Mechanism Design for Team Formation
Source: arXiv:1501.00715 source file (2015-01-04)
Supplement: Supplementary file 1 [file appendixtf.pdf]

## Appendix

### Team Size Constraints that Admit a Feasible Allocation

Some tuples  $(N, \underline{k}, \bar{k})$  are not feasible, meaning that it is not possible to divide  $|N|$  players into coalitions with sizes in  $[\underline{k}, \bar{k}]$ . Recall that we require by definition  $1 \leq \underline{k} \leq \bar{k} \leq |N|$ . For a minimal example, it is not possible to divide 3 players into coalitions with  $\underline{k} = 2, \bar{k} = 2$ .

**Observation 1.** *A tuple  $(N, \underline{k}, \bar{k})$  is feasible if and only if:  $\underline{k}$  divides  $|N|$ ,  $\bar{k}$  divides  $|N|$ , or  $(|N| \setminus \underline{k}) > (|N| \setminus \bar{k})$ , where  $\setminus$  signifies integer division.*

### Computing Social Welfare-Maximizing Allocation

In order to find a social welfare maximizing solution, we formulate the problem as an MIP and solve it using CPLEX. We are given a feasible mechanism design problem as  $(N, \succ, \underline{k}, \bar{k})$ , where either  $\underline{k} = \bar{k}$ , or  $\underline{k} + 1 = \bar{k}$  and neither  $\underline{k}$  nor  $\bar{k}$  divides  $|N|$ . Let  $T$  equal the number of teams that results when as many teams of size  $\bar{k}$  as possible are formed, the rest being of size  $\underline{k}$ .

We introduce a matrix  $x \in \{0, 1\}^{T \times |N|}$ , where each row corresponds to one team, and the 1 values in the row indicate which agents are on that team. We also introduce a dummy variable,  $S \in \{0, 1\}^{T \times |N| \times |N|}$ , where  $S_{tij} = 1$  if agents  $i$  and  $j$  are both on team  $t$ , otherwise 0.  $S'_{ij} \in \{0, 1\}^{|N| \times |N|}$  is 1 if and only if agents  $i$  and  $j$  are on the same team, and is the sum over  $t$  values of  $S_{tij}$  for  $i$  and  $j$ .

The MIP for maximize social welfare is then:

$$\begin{aligned} \max_x : & \sum_{i=1}^{|N|} \sum_{j=i+1}^{|N|} S'_{ij}(u_{ij} + u_{ji}) \\ \text{subject to:} \\ & x \in \{0, 1\}^{T \times |N|} \\ & S \in \{0, 1\}^{T \times |N| \times |N|} \\ & S' \in \{0, 1\}^{|N| \times |N|} \\ & 2S_{tij} \leq x_{ti} + x_{tj} : \forall t, i, j \\ & S_{tij} \geq x_{ti} + x_{tj} - 1 : \forall t, i, j \\ & S'_{ij} = \sum_{t=1}^T S_{tij} : \forall i, j \\ & \underline{k} \leq \sum_{j=1}^{|N|} x_{tj} \leq \bar{k} : \forall t \\ & \sum_{t=1}^T x_{tj} = 1 : \forall j \end{aligned}$$

We implemented a second version of the maximize social welfare MIP, which appears to run much faster. In this version, a matrix  $x \in \{0, 1\}^{|N| \times |N|}$  has a 1 in row  $i$  for each agent on the team of agent  $i$ . We require that  $x_{ij} = x_{ji}$  so

that demands are reciprocal. We also require that each agent demand itself, so  $x_{ii} = 1$ . Each team size must be in  $[\underline{k}, \bar{k}]$ , so the sum of each row of  $x$  must be in this range. Finally, we require that any two rows in  $x$  either not have a 1 in any of the same columns, or must be identical; this means that if some agent  $i$  appears on two teams (i.e., in two rows), those teams must contain exactly the same agents.

$$\begin{aligned} \max_x : & \sum_{i=1}^{|N|} \sum_{j=1}^{|N|} x_{ij} u_{ij} \\ \text{subject to:} \\ & x \in \{0, 1\}^{|N| \times |N|} \\ & x_{ii} = 1 : \forall i \\ & x_{ij} - x_{ji} = 0 : \forall i, j \\ & \underline{k} \leq \sum_{j=1}^{|N|} x_{ij} \leq \bar{k} : \forall i \\ & x_{ij} + x_{i'j} + x_{ij'} - x_{i'j'} \leq 2 : \forall i, i' \neq i, j, j' \neq j \end{aligned}$$

### Proof of Proposition 1

Consider a hedonic game with 6 agents,  $\{A, B, C, D, E, F\}$ ,  $\underline{k} = 3, \bar{k} = 3$ , so that two equal-size coalitions must be formed. The agents' additive separable preferences are encoded in Table 7.

|   | A | B | C | D | E | F |
|---|---|---|---|---|---|---|
| A | x | 0 | 1 | 2 | 4 | 8 |
| B | 8 | x | 4 | 2 | 1 | 0 |
| C | 8 | 0 | x | 4 | 2 | 1 |
| D | 8 | 1 | 0 | x | 4 | 2 |
| E | 8 | 2 | 1 | 0 | x | 4 |
| F | 8 | 4 | 2 | 1 | 0 | x |

Table 7: Each row  $i$  encodes the additive separable value for agent  $i$  of each other agent.

No partition of these agents into two teams of size 3 gives every agent envy bounded by a single good. To see this, consider that each agent other than  $A$  has a bliss point on a team with  $A$  and one other agent, where the second agent is  $C$  for agent  $B$ ,  $D$  for agent  $C$ , and so on until "wrapping around" with  $B$  for agent  $F$ . Three of the agents will not be on a team with agent  $A$ , and at least one of these agents, say agent  $i$ , will not be on a team with its second-favorite agent either. Some other agent  $j$  must then be on a team with the two most preferred agents of the player  $i$ . By construction, player  $i$  is on a team of value 3 or less, while the team of agent  $j$  has value 12 to agent  $i$ , and value 4 to agent  $i$  with its more valuable player (player  $A$ ) removed. Therefore, envy cannot be bounded by a single good for all agents.  $\square$

**Maximin Share Guarantee** A maximin share for an agent is the agent's least preferred bundle in a *maximin split* for

the agent, which is a partition of all goods into one bundle per agent that maximizes the utility of the least valuable bundle. Note that envy-freeness implies proportionality, and proportionality implies maximin shares (Procaccia and Wang 2014). We introduce a modified version of the maximin share guarantee in our setting, the *maximin share guarantee for team formation*. A coalition structure in a hedonic game provides maximin shares for hedonic games, if each agent weakly prefers its bundle of other agents to its maximin share. Given  $(N, \succ_i, \underline{k}, \bar{k})$ , consider all partitions of the agents  $N$  with coalition sizes in  $[\underline{k}, \bar{k}]$ . A maximin split for agent  $i$  is any such partition that maximizes the value for  $i$  of the least preferred coalition containing  $i$ , which would result from swapping  $i$  with some agent  $j$ , where  $j$  may equal  $i$ . A maximin share is the least preferred coalition in a maximin split. This definition of the maximin share guarantee preserves a useful property of the guarantee for multi-unit assignment, which is that an agent may be assigned one of  $|N|$  bundles from its maximin split.

The maximin share guarantee for ASHG with non-negative values is trivially satisfiable for  $\bar{k} = |N|$ : If the grand coalition is assigned, every agent's payoff is maximized, so envy-freeness is achieved. The maximin share guarantee for ASHG with non-negative values is also trivially satisfiable for  $\bar{k} = 2$ . In the maximin split for an agent with  $\bar{k} = 2$ , all agents are grouped in pairs (assuming  $|N|$  is even), and the agent's maximin share is the pair with its least favorite other agent. Thus, any grouping of the agents into pairs satisfies the maximin share guarantee.

**Proposition 7.** *For some ASHGs with non-negative values,  $\bar{k} \geq 3$ , and  $\bar{k} < |N|$ , the maximin share guarantee for hedonic games is not satisfiable. As a result, proportionality and envy-freeness are not satisfiable either in such cases.*

*Proof.* Consider a hedonic game with 6 agents,  $\{A, B, C, D, E, F\}$ ,  $\underline{k} = 3$ ,  $\bar{k} = 3$ , so that two equal-size coalitions must be formed. The agents' additive separable preferences are encoded in Table 8.

|   | A | B | C | D | E | F |
|---|---|---|---|---|---|---|
| A | x | 1 | 0 | 2 | 3 | 2 |
| B | 2 | x | 1 | 0 | 3 | 2 |
| C | 2 | 2 | x | 1 | 0 | 3 |
| D | 1 | 2 | 2 | x | 2 | 1 |
| E | 0 | 2 | 3 | 1 | x | 2 |
| F | 2 | 1 | 2 | 2 | 1 | x |

Table 8: Each row  $i$  encodes the additive separable value for agent  $i$  of each other agent.

It is easy to see that in the game described above, each agent's maximin share for hedonic games has value 3. Furthermore, any of the 10 possible partitions of the agents into two equal-size groups leaves some agent with a coalition value of 2 or less. Therefore, no partition for this game provides every agent with a maximin share. In consequence, no partition for this game is proportional or envy-free either.  $\square$

## Proof of Proposition 2

Random serial dictatorship for team formation is strategyproof, meaning that it is a dominant strategy for each agent to reports its true values for other agents, regardless of the other agents' reports. Consider that each agent affects the allocation returned by RSD only if the agent is a "team captain," based on the serial order over players and the choices of earlier team captains. Therefore, if an agent is not a team captain, the agent's report makes no difference. If an agent is a team captain, the agent is assigned its most preferred team based on the remaining players, team size constraints, and the agent's reported preferences. Therefore, it is a dominant strategy for the agent to report its true preferences.

Random serial dictatorship is ex post Pareto efficient for ASHGs with strict preferences over teams (i.e., without indifferences over teams). The first "team captain" is assigned its strictly most preferred team, of the largest feasible team size. Thus, for non-negatively values ASHGs, no other agent could swap or take agents from the first captain's bundle without decreasing its value to the captain. The same argument holds, by induction, for later team captains. Thus, the allocation from RSD is ex post Pareto efficient.

Random serial dictatorship for ASHGs is not envy-free, because for some ASHG instances, no envy-free allocation exists, as shown in Proposition 7.  $\square$

## Proof of Proposition 3

The Harvard Business School draft for ASHGs is not envy-free, because for some ASHG instances, no envy-free allocation exists, as shown in Proposition 7.

The HBS draft for team formation is not ex post Pareto efficient. For a counter-example, consider the following ASHG, with  $\underline{k} = \bar{k} = 3$  and player order  $(A, B, C, D, E, F)$ , such that  $A$  and  $B$  will be the team captains. The agent preferences are encoded in Table 9.

|   | A | B | C  | D | E | F |
|---|---|---|----|---|---|---|
| A | x | 1 | 8  | 0 | 6 | 4 |
| B | 1 | x | 10 | 0 | 5 | 3 |
| C | 0 | 8 | x  | 5 | 4 | 2 |
| D | 0 | 8 | 5  | x | 4 | 2 |
| E | 8 | 0 | 5  | 4 | x | 2 |
| F | 8 | 0 | 5  | 4 | 2 | x |

Table 9: Each row  $i$  encodes the additive separable value for agent  $i$  of each other agent.

In this example, the following selections are made in the HBS draft.  $A$  selects  $C$ ,  $B$  selects  $E$ ,  $B$  selects  $F$ , and then  $A$  selects  $D$ . The resulting allocation is  $\{(ACD), (BEF)\}$ . This allocation is not ex post Pareto efficient, because all the agents would prefer the allocation  $\{(AEF), (BCD)\}$ .

The HBS draft for team formation is not strategyproof. Consider a minimal-size example of an ASHG with non-negative values, where the HBS draft is not strategyproof. Let  $N = \{A, B, C, D, E, F\}$ ,  $\underline{k} = 3$ , and  $\bar{k} = 3$ . The players' additive separable values to each other are encoded in the Table 10.

|           | <i>A</i> | <i>B</i> | <i>C</i> | <i>D</i> | <i>E</i> | <i>F</i> |
|-----------|----------|----------|----------|----------|----------|----------|
| <i>A</i>  | x        | 5.0      | 4.9      | 7.0      | 0.2      | 0.0      |
| <i>A'</i> | x        | 5.0      | 6.0      | 7.0      | 0.2      | 0.0      |
| <i>B</i>  | 0.0      | x        | 1.1      | 1.6      | 1.2      | 1.3      |
| <i>C</i>  | 0.0      | 1.1      | x        | 1.6      | 1.2      | 1.3      |
| <i>D</i>  | 0.0      | 1.1      | 1.6      | x        | 1.2      | 1.3      |
| <i>E</i>  | 0.0      | 1.1      | 1.6      | 1.2      | x        | 1.3      |
| <i>F</i>  | 0.0      | 1.1      | 1.6      | 1.2      | 1.3      | x        |

Table 10: Each row  $i$  encodes the additive separable value for agent  $i$  of each other agent. Row  $A'$  shows the false report of agent  $A$ .

In the ASHG shown in Table 10, agent  $A$  gets greater utility by misreporting its preferences as in  $A'$  for 24 serial orders over the players, and never receives worse utility than when reporting  $A$ . In each of the 24 cases where  $A$  gains by reporting  $A'$ , utility improves from 5.2 to 9.9, as the received team shifts from  $(ABE)$  to  $(ABC)$ . This occurs when the first player to choose is  $A$  and the second is  $D$ . Therefore, the HBS draft is not strategyproof, because in the example shown, player  $A$  gets better expected utility by misreporting its preferences.  $\square$

#### Proof of Proposition 4

Consider a minimal-size example of an ASHG with non-negative values, where the OPOP draft is not strategyproof. Let  $N = \{A, B, C, D, E, F\}$ ,  $\underline{k} = 3$ , and  $\bar{k} = 3$ . The players' additive separable values to each other are encoded in the Table 11.

|           | <i>A</i> | <i>B</i> | <i>C</i> | <i>D</i> | <i>E</i> | <i>F</i> |
|-----------|----------|----------|----------|----------|----------|----------|
| <i>A</i>  | x        | 5.0      | 4.9      | 7.0      | 0.2      | 0.0      |
| <i>A'</i> | x        | 5.0      | 6.0      | 7.0      | 0.2      | 0.0      |
| <i>B</i>  | 0.0      | x        | 1.1      | 1.6      | 1.2      | 1.3      |
| <i>C</i>  | 0.0      | 1.1      | x        | 1.6      | 1.2      | 1.3      |
| <i>D</i>  | 0.0      | 1.1      | 1.6      | x        | 1.2      | 1.3      |
| <i>E</i>  | 0.0      | 1.1      | 1.6      | 1.2      | x        | 1.3      |
| <i>F</i>  | 0.0      | 1.1      | 1.6      | 1.2      | 1.3      | x        |

Table 11: Each row  $i$  encodes the additive separable value for agent  $i$  of each other agent. Row  $A'$  shows the false report of agent  $A$ .

The OPOP draft is a randomized allocation mechanism, which works by uniformly randomly choosing a permutation of the players, then acting deterministically based on that order. Strategyproofness for a randomized mechanism means that a player's expected payoff is maximized by truthful reporting, regardless of other players' actions. To show that the OPOP draft is not strategyproof, it suffices to show that player  $A$  gains in expected payoff, based on the true preferences in row  $A$  of the table, by misreporting its preferences as in row  $A'$  in the table, if other players report their preferences as displayed in the table.

The example game has 6 players, so there are  $6! = 720$  permutations, and 720 equally likely outcomes from the OPOP draft, some of which are identical in their allocations.

It turns out that the payoff for player  $A$  is better when reporting  $A'$  instead of  $A$  for 18 of 720 permutations, and worse in 6 others. Specifically, player  $A$  performs better by lying if and only if the order of the first three players to choose is  $(ADB)$ ,  $(ADE)$ , or  $(ADF)$ . Player  $A$  does worse by reporting  $A'$  if and only if the order of the first three players is  $(ADC)$ . After factoring in the value of the resulting allocations to player  $A$ , it results that the expected value of defecting to  $A'$  is 0.08 utils per game. Thus, the OPOP draft is not strategyproof.

The One-Player-One-Pick draft for ASHG is not envy-free, because for some ASHG instances, no envy-free allocation exists, as shown in Proposition 7.

The OPOP draft for ASHG is not ex post Pareto efficient, as shown in the following minimal example. Let  $N = \{A, B, C, D, E, F\}$ ,  $\underline{k} = 3$ , and  $\bar{k} = 3$ . Let the serial order of the players be alphabetical, so  $A$  selects first, and so on. The players' additive separable values to each other are encoded in Table 12.

|          | <i>A</i> | <i>B</i> | <i>C</i> | <i>D</i> | <i>E</i> | <i>F</i> |
|----------|----------|----------|----------|----------|----------|----------|
| <i>A</i> | x        | 2        | 10       | 9        | 6        | 0        |
| <i>B</i> | 0        | x        | 10       | 9        | 2        | 6        |
| <i>C</i> | 0        | 10       | x        | 2        | 6        | 9        |
| <i>D</i> | 10       | 0        | 2        | x        | 6        | 9        |
| <i>E</i> | 10       | 0        | 2        | 6        | x        | 9        |
| <i>F</i> | 0        | 10       | 2        | 6        | 9        | x        |

Table 12: Each row  $i$  encodes the additive separable value for agent  $i$  of each other agent.

In the example ASHG in Table 12, the following selections are made, in order. Team captain  $A$  selects  $C$ , team captain  $B$  selects  $D$ ,  $C$  (already teamed with  $A$ ) selects  $F$ , and as a result  $D$  (already teamed with  $B$ ) must select  $E$ . This produces the allocation  $\{(ACF), (BDE)\}$ . Every player would receive greater utility from the alternative allocation  $\{(ADE), (BCF)\}$ . Therefore, the OPOP draft is not ex post Pareto efficient.  $\square$

#### Details of A-CEEI-TF

Each agent reports to the mechanism the additive separable utility it gains from each other agent. The mechanism uses these reports to derive which affordable bundle of other agents each agent demands, given each agent's budget and price. The total utility for an agent  $i$  of a bundle of other agents of size in  $[\underline{k} - 1, \bar{k} - 1]$ , is the sum of the utilities for agent  $i$  of the agents in that bundle. The clearinghouse will provisionally assign agent  $i$  the bundle of highest utility for  $i$  that it can afford, or the empty bundle if it cannot afford any bundle of legal size.

Just as in combinatorial matching, we cannot in general hope for an exact market clearing solution (and, consequently, an exact CEEI) in our setting:

**Proposition 8.** *There exist team formation settings where no price and budget vectors  $(p, b)$  exist that induce exact market clearing.*

*Proof.* We define *exact market clearing for hedonic games* to mean that when each agent is allocated its favorite bundle of other agents that is affordable:

- Each agent is assigned to a coalition with size in  $[\underline{k}, \bar{k}]$ , including itself in the coalition size.
- For any two distinct agents  $i$  and  $j$ ,  $i$  demands  $j$  if and only if  $j$  demands  $i$ .

This result marks a distinction from the course allocation problem, where with sufficiently unequal budgets, some price vector must exist that induces exact market clearing (Budish 2011).

*Example.* Consider a hedonic game with 4 agents,  $\{A, B, C, D\}$ , with  $\underline{k} = 2$  and  $\bar{k} = 2$ . The agents' additive separable preferences are encoded in Table 13.

|   | A | B | C | D |
|---|---|---|---|---|
| A | x | 2 | 1 | 0 |
| B | 0 | x | 2 | 1 |
| C | 1 | 0 | x | 2 |
| D | 2 | 1 | 0 | x |

Table 13: Each row  $i$  encodes the additive separable value for agent  $i$  of each other agent.

In the example in Table 13, only two allocations must be considered, due to symmetry:  $\{\{A, B\}, \{C, D\}\}$  and  $\{\{A, C\}, \{B, D\}\}$ .

In order for the market to clear as  $\{\{A, B\}, \{C, D\}\}$ , each agent must be able to afford its assigned partner, and each agent must not be able to afford any other agent that it prefers. If we assume the market clears in this way, the resulting inferences produce an impossible conclusion:

$$p_A \leq b_B < p_C \leq b_D < p_A$$

A similar conclusion can be drawn from the other allocation,  $\{\{A, C\}, \{B, D\}\}$ . We find that no  $(b, p)$  induces exact market clearing for this game, no matter how unequal the agents' budgets in  $b$  are.  $\square$

Define the price update error as

$$z(p)_j = (1 + \epsilon - (\epsilon/\bar{b})p_j)D_j - U_j.$$

Since exact market clearing is not feasible, we make use of a relaxation. We define a notion of *relaxed market clearing*, which we will use in our search for approximately market-clearing prices. This form of market clearing allows a good on the market to be under-demanded if and only if its price is 0. We adapt this relaxed form of market clearing from Budish (Budish 2011). In relaxed market clearing:

- Each agent is assigned to a coalition with size in  $[\underline{k}, \bar{k}]$ , including itself in the coalition size, unless the agent has price 0, in which case it may alternatively be assigned the team containing only itself.
- For any two distinct agents  $i$  and  $j$ ,  $i$  demands  $j$  if and only if  $j$  demands  $i$ .

**Proposition 9.** *There exists a point  $p^*$  in price space  $\mathcal{P}$ , for which a convex combination of the error terms  $z(p')$  induced by some set of prices near  $p^*$  equals the zero vector, as in relaxed market clearing.*

*Proof.* The proposition can be proved through a straightforward adaptation of the proof of Theorem 1 in Budish (Budish 2011). First we note that any fixed point of  $f(\cdot)$  induces relaxed market clearing. Furthermore, the price space  $\tilde{\mathcal{P}}$  is compact, convex, and closed under  $f(\cdot)$ . We introduce a function  $F(\tilde{p})$  that takes the convex hull of all values  $f(\tilde{p}')$ , for  $\tilde{p}'$  approaching in the limit but not equal to  $\tilde{p}$ .

Lemma 2.4 of Cromme and Diener is useful here (Cromme and Diener 1991). Take any space  $\mathcal{X}$  that is a non-empty, compact, convex subset of  $\mathbb{R}^d$ , and any function  $f : \mathcal{X} \rightarrow \mathcal{X}$ , such that  $\mathcal{X}$  is closed under  $f$ . Define  $H_f : \mathcal{X} \rightarrow S$ ,  $S \subset \mathcal{X}$ , to be the function that takes any  $x$  in  $\mathcal{X}$  and yields the set:

$$\{y \in \mathcal{X} \mid \exists \text{ a sequence } x_i \rightarrow x, x_i \neq x : f(x_i) \rightarrow y\}$$

Lemma 2.4 of Cromme and Diener states that for any such function  $f$ , there exists a point  $x^* \in \mathcal{X}$  such that  $x^*$  is in the convex hull of  $H_f(x^*)$ .

We can apply Cromme and Diener's result to  $F(\cdot)$ , because the auxiliary price space  $\tilde{\mathcal{P}}$  is non-empty, compact, convex, and closed under  $f(\cdot)$ , and  $F(\cdot)$  is defined as the convex hull of Cromme and Diener's  $H_f$ . Therefore, as shown in Cromme and Diener, Kakutani's fixed point theorem implies that  $F(\cdot)$  has a fixed point  $\tilde{p}^* \in \tilde{\mathcal{P}}$ . Thus, a convex combination of the error terms  $z(p')$  near  $t(\tilde{p}^*)$  yields relaxed market clearing.  $\square$

The fixed point result in Proposition 9 implies that for prices  $p'$  in the neighborhood of the truncation of a fixed point  $\tilde{p}^*$  of the price update function, induced market clearing error will be low. Therefore, we will likely be able to find price vectors that yield low market clearing error by iteratively applying  $f(\cdot)$  to its own output, until an apparent fixed point is approached.

## Proof of Proposition 5

First, we show that auxiliary price space  $\tilde{\mathcal{P}}$  is closed under  $f(\cdot)$ . The range of  $z(p)_j$  for  $p \in \mathcal{P}$  is  $[-1, (|N'| - 1)(1 + \epsilon)]$ . Thus, assuming  $\epsilon$  is small,  $|z(p)_j|/|N'| < 1$ . Therefore, it is easy to see that auxiliary price space  $[-1, 1 + \bar{b}]^{|N'|}$  is closed under  $f(\cdot)$ .

Next, we show that if  $\tilde{p} \in \tilde{\mathcal{P}}$  is a fixed point of  $f(\cdot)$ , then  $p = t(\tilde{p})$  must induce relaxed market clearing.

Each agent price  $p_j$  in  $p = t(\tilde{p})$  must either equal 0, equal  $\bar{b}$ , or be in  $(0, \bar{b})$ .

If  $p_j = \bar{b}$ , then no agent can afford to demand agent  $j$ , so  $UND_j = 1$  and  $IURQ_j = 0$ , implying that  $z(p)_j$  is negative, so  $p_j$  cannot be a fixed point. If  $p_j$  has been truncated by  $t(\cdot)$ , this would reduce it, and  $z(\cdot)$  further reduces it.

If  $p_j = 0$ , then if there is  $IURQ_j > 0$  and  $UND_j = 0$ , the net effect of  $z(p)_j$  is to increase  $p_j$ , and if  $p_j$  has been truncated, then that would have increased  $p_j$  also; so with

or without truncation,  $p_j$  would not be a fixed point if it had positive  $IURQ$  but not  $UND$ . If  $p_j = 0$  and  $IURQ = 0$ , then under-demand for  $j$  is allowed because the price of  $j$  is zero, so this does not violate relaxed market clearing.  $IURQ_j$  and  $UND_j$  cannot both be positive, because if there is incoming demand, there is no under-demand by definition.

If  $p_j \in (0, \bar{b})$ , and  $p_j$  is part of a fixed point  $p$ , then  $UND_j = 0$  and  $IURQ_j = 0$ , because by definition, they cannot both be positive at once.  $\square$

### Proof of Proposition 6

First, we sketch out a proof of strategyproofness-in-the-large.

Any individual agent in the continuum economy, being zero-measure, has no influence on the approximate equilibrium price vector arrived at by update function  $f(\cdot)$ , at any iteration of the A-CEEI-TF mechanism. Therefore, the only effect the agent can have on the outcome is that, if the agent is randomly selected to choose its favorite affordable bundle of free agents that leaves a feasible subproblem, the agent's reported preferences determine which bundle the agent is assigned. Thus, it is a dominant strategy for the agent to report its true preferences, so that in this case the agent will be assigned its most preferred allowable team.  $\square$

Now we deal with approximate envy-freeness.

Consider a team formation problem where A-CEEI-TF yields exact market clearing with the same allocation at each stage. If all agent budgets were equal, then the result would be envy-free. To see this, consider that each agent's allocation by A-CEEI-TF in such cases is the same as the allocation induced by prices in the initial round of price search. In this initial round, every agent is able to afford the allocation of every other agent, because all agent budgets are equal, and each agent demands its own bundle rather than the bundle demanded by some other agent, because there is exact market clearing. Because the final allocations returned are the same as those induced by the initial prices, no agent must envy any other in the final allocation.

More generally, consider the same setting but without equal budgets. That is, consider an ASHG with non-negative values and team size constraints, where A-CEEI-TF yields exact market clearing with the same allocation at each stage. Recall that all agents' budgets are in the range  $[1, \bar{b}]$ , where  $\bar{b} = 1 + (1/|N|)$ . Because  $1 \leq \bar{k} \leq |N|$ , this implies that  $\bar{b} \leq 1 + (1/\bar{k})$ .

No agent  $i$  can envy another agent  $j$  in its own bundle, because  $j$ 's allocation (excluding the costs of  $i$  and  $j$ ) costs weakly less than the allocation of  $i$  (excluding the cost of  $i$ ), as all agent prices are non-negative, so  $i$  could afford the bundle of other agents that  $j$  receives (the team of agent  $i$ , excluding agents  $i$  and  $j$ ).

Assume for a contradiction that  $i$  has envy for agent  $j$  that is not bounded by a single good. Note that  $i$  and  $j$  must be assigned to distinct teams. Let  $k'$  be the number of other agents in  $j$ 's bundle,  $k' < \bar{k}$ . Let  $j_1$  be the first other agent in  $j$ 's bundle, and so on through  $j_{k'}$ .

Let  $p$  be the exact market clearing prices that are found in the first stage of the A-CEEI-TF mechanism. Let  $x$  be the allocation that is induced by the mechanism, which we have

assumed to be consistent across all stages of the price search.  $x_i$  is then a vector in  $\{0, 1\}^{|N|}$  that has a 1 for each agent on the same team as agent  $i$ . For convenience in calculating the cost of the team for agent  $i$ , we let  $x_{ii} = 0$  for all  $i$ , because an agent is not required to pay the cost of teaming with itself. Let  $(x_i \setminus \{j\})$  be a vector equivalent to  $x_i$ , but with  $x_{ij}$  set to 0.

$p \cdot (x_j \setminus \{j_r\}) > b_i : \forall r \in \{1, \dots, k'\}$ . This is because if agent  $i$ 's envy for agent  $j$  is not bounded by a single good, agent  $i$  must not be able to afford any subset of  $j$ 's bundle created by removing one item (and excluding agent  $j$ ).

$(k' - 1)p \cdot x_j > k'b_i$ . This comes from adding the L.H.S. and R.H.S. of the  $k'$  inequalities above, where the subtracted items from  $x_j$  cancel to produce one fewer complete  $x_j$ .

$b_j \geq p \cdot x_j$ , because agent  $j$  can afford its own bundle.

$(k' - 1)b_j > k'b_i$ . Replacing  $p \cdot x_j$  with  $b_j$  in the inequality above.

$b_j/b_i > k'/(k' - 1)$ .

Recall that  $\bar{b} \leq 1 + (1/\bar{k})$ , and  $\bar{k} \geq 1$ , meaning that  $\bar{b} \leq 1 + (1/(\bar{k} - 1))$ . This implies that  $\bar{k}/(\bar{k} - 1) \geq \bar{b}$ .

$\bar{k} > k'$ , which implies  $k\bar{k}' - \bar{k} < k\bar{k}' - k'$ . So  $\bar{k}(k' - 1) < k'(\bar{k} - 1)$ . This means  $\bar{k}/(\bar{k} - 1) < k'/(k' - 1)$ .

$b_j/b_i > k'/(k' - 1) > \bar{k}/(\bar{k} - 1) > \bar{b}$ .

$b_j/b_i > \bar{b}$ .

This contradicts the claim that all budgets are  $\in [1, \bar{b}]$ . Therefore, envy must be bounded by a single good in an ASHG with non-negative values and team size constraints, where A-CEEI-TF yields exact market clearing with the same allocation at each stage.  $\square$

### A-CEEI-TF Implementation

Unlike the alternative mechanisms, A-CEEI-TF is far from straightforward to implement. Below we describe an implementation which uses ideas from Othman, Sandholm, and Budish (2010).

To run the A-CEEI-TF mechanism, we used a modified form of the procedure described by Othman, Sandholm, and Budish, which alternates tabu search and mixed-integer program (MIP) solving until an approximate fixed point is found (Othman, Sandholm, and Budish 2010). The mechanism starts by randomly assigning approximately equal budgets to the agents  $\in (100, 100 + 100/|N|)$ , and setting prices for all agents to be equal to the minimum agent budget divided by the maximum number of agents that can be legally demanded,  $(\bar{k} - 1)$ . Based on the random order of players, the next unselected player in order is allowed to select its favorite affordable bundle of unselected players, of legal size and that leaves a feasible subproblem. Before a player can make this selection, the tabu search-MIP hybrid algorithm is run to assign the prices to remaining agents.

Each time the price search procedure is called, 20 iterations of tabu search are run. For a given iteration, the current price vector is "expanded" to yield up to  $5|N| + 5$  new price vectors, each of which is evaluated in terms of its relaxed market clearing error.

The new price vectors are generated as either unilateral deviations from the current price vector, or moves in the direction of the "gradient," or  $z(\cdot)$ . The gradient neighbors of

$p$  are generated by moving in the direction of  $z(p)$ , for each of the step sizes (10.0, 5.0, 1.0, 0.5, 0.1), where the step size is just the  $L_2$ -norm of the change in  $p$ . For each agent  $j$ , we generate unilateral neighbors of  $p$  by setting the agent's price to 0 if  $z(p)_j \leq 0$ , otherwise by increasing the agent's price by each of (1.0, 0.5, 0.1, 0.05, 0.001). Any neighbor prices outside of  $[0, \bar{b}]$  are truncated to this range.

Each neighbor price vector of the previous price  $p$  is evaluated for its market clearing error, using an MIP solver to determine which bundle of other agents each agent would demand at those prices. We used CPLEX v12.5, with Concert bindings for Java, to solve each MIP. Market clearing error for a price vector  $p$  is defined as the  $L_2$ -norm of  $z(p)$ .

A "step" of the tabu search entails moving from the previous price vector to the price vector of lowest error among the neighbors, that is not in the tabu list (a list of the previously visited price vectors). After 20 iterations, the visited price vector that produced the lowest (best) market clearing error is returned.

To find which bundle of other agents an agent  $j$  will demand, given a set of legal bundle sizes that leave feasible subproblems, we first break the legal bundle sizes into groups of consecutive integers. For example, if  $\underline{k} = 2, \bar{k} = 4$ , and there are 4 agents remaining including the "self" agent, it is not legal for the agent to demand 2 other agents for a bundle of size 3, even though  $3 \in [2, 4]$ , because this does not leave a feasible subproblem. So in this case we would first break up the problem into two distinct MIPs, one with  $\underline{k} = \bar{k} = 2$ , the other with  $\underline{k} = \bar{k} = 4$ . The agent's preferred bundle from the union of the MIP result bundles would then be returned as the agent's demand.

Now we have a price vector  $p$  over the  $M$  other remaining agents and a continuous range of integers that are legal bundle sizes,  $\{\underline{k}, \underline{k} + 1, \dots, \bar{k}\}$ . The demand of agent  $j$  with budget  $b_j$  is:

$$\begin{aligned} \max_c : & \sum_{i=1}^{|M|} c_i u_j(i) \\ \text{subject to:} \\ & c \in \{0, 1\}^{|M|} \\ & \sum_{i=1}^{|M|} c_i p_i \leq b_j \\ & \underline{k} - 1 \leq \sum_{i=1}^{|M|} c_i \leq \bar{k} - 1 \end{aligned}$$

### Data Sets: Preference Similarity

The four classes of data set we analyze differ most saliently in their number of agents,  $|N|$ , and in the degree of similarity among the preferences of their agents. For example, Random-similar agents largely agree on which other agents are most valuable, while Random-scattered agents have little agreement. Differences in degree of preference similarity lead to marked differences in the performance outcomes of the various mechanisms.

As our measure of agent preference similarity in a data set, we let  $\mathcal{C}$  equal the mean cosine similarity among all pairs of distinct agents in that data set. Because each agent assigns itself a value of 0 or undefined, we take the cosine similarity between agents  $i$  and  $j$  only over their values for agents in  $N \setminus \{i, j\}$ :

$$\begin{aligned} u_{i-j} &= u_i \setminus \{u_{ii}, u_{ij}\} \\ \mathcal{C} &= \frac{\sum_{i=1}^{|N|} \sum_{j=i+1}^{|N|} \frac{u_{i-j} \cdot u_{j-i}}{\|u_{i-j}\| \|u_{j-i}\|}}{(|N|^2 - |N|)/2} \end{aligned}$$

In Table 14, we present the mean cosine similarity for each data set we discuss in this paper. Higher cosine similarities indicate greater agreement among agents about the relative values of other agents. We also show the number of agents in each data set.

|                     | $\mathcal{C}$ | $ N $ | $\underline{k}$ | $\bar{k}$ |
|---------------------|---------------|-------|-----------------|-----------|
| Random-similar 20   | 0.914         | 20    | 5               | 5         |
| Random-scattered 20 | 0.499         | 20    | 5               | 5         |
| Newfrat             | 0.877         | 17    | 4               | 5         |
| Freeman             | 0.551         | 32    | 5               | 6         |

Table 14: Mean cosine similarity over all pairs of distinct agents, number of agents, minimum team size, and maximum team size. For random data set classes,  $\mathcal{C}$  as shown is the mean over 20 randomly generated instances of the data set class.
